# Supplementary material for: SMT-Based Dynamic Multi-Robot Task Allocation
Source: arXiv:2403.11737 source file (2024-03-18)
Supplement: Supplementary file 1 [file sketch_appendix_no_statements.tex]

\section{Soundness}

\subsection{Proof Sketch of Lemma 1}
Plan building is deterministic, so per assignment, we will only get one possible $\plan_0$. We argue that action point times are strictly monotonically increasing. Because the task start and end literals can only be assigned one time, they can only be assigned one action point, so pick and drop actions occur once. For load constraints, we connect the load of an action sequence to the load at each action point and can say that is constrained by construction. Other aspects are true by construction.

\subsection{Proof Sketch of Lemma 2}
By Lemma \ref{lemma:consistent_action_seq}, we know each agent's action sequence is consistent. By construction, each task must be assigned an agent id and will only be assigned one agent because agent ids are unique. An assignment implies that an agent starts (picks up) the task which implies the agent also ends (drops) the task. The duration of every pick or drop element in the action sequence is equal to the time of a corresponding action point. With this we show the duration constraints are satisfied.

\subsection{Proof Sketch of Lemma 3}
For each agent, action sequences are constructed deterministically from an assignment. $\modeloutput_{j+1}$ is constrained to have $\dptuple = \modeloutput_j(\dptuple)$ $\forall d = 1, \ldots, d'-1$ for some $d' = 1, \ldots, D$. Thus, some length prefix in each action sequence is equivalent. In SavePastState(), we either add constraints until the end of the relevant action points ($d + 1 < D \wedge \nextdpid = n$), making the new prefix equal to the old after which we add a wait by construction. In the other, we continue until the time of the action point is $\geq t_j$, which will satisfy the other option for an updated plan. By construction, the last action will be a pick or a drop.

\subsection{Proof Sketch of Lemma 4}

The statements from the proof of Lemma \ref{lemma:consistent_action_seq} hold except that a wait action can now exist. $\wait \cap \move = \emptyset$, so there will still not be two adjacent moves. The addition of a wait either shifts both pick and drop points for a task or shifts just the drop, so drop will still be after pick. Waits are not directly included in the action point encoding, so times are still unique. Therefore, pick and drop actions still only occur once. Similarly, waits will not affect the load values of the action points.

\subsection{Proof Sketch of Lemma 5}
We know by Lemma \ref{lemma:updated_consistency} that the updated action sequence is consistent. The statements in Lemma \ref{lemma:completed_tasks} hold for the new set of tasks.  

\section{Completeness}

\subsection{Proof Sketch of Lemma 6}
As shown in Lemma \ref{lemma:consistent_action_seq}, pick and drop ids will only occur once per task in an agent's assignment in a satisfying $\modeloutput$. By construction, action point ids must be either $\dpid = \agent$ or $\dpid \geq \numagents \wedge \dpid < 2\numtasks + \numagents$. Therefore, for an agent $\agent$, the maximum number of action points that can be assigned to a value other than $\agent$ is $2\numtasks$. Adding in the constrained 0th action point, the total is $2\numtasks + 1 = D_{max}$ where $\dpid = n$ for $d = d' \geq D_{max}$. By construction $\dptime[\agent][d']=max\_time$ and $\dpload[\agent][d'] = 0$ because picked up tasks must have been dropped off beforehand. Therefore, adding an extra action point does not add new free variables, so an unsat result cannot turn sat by adding more action points.

\subsection{Proof Sketch of Lemma 8}
An action point $d$ is free if it is not constrained to have $\dpid = \agent$.  By inspection we see that the while loop in Lines \ref{line:dp_increase1} and \ref{line:dp_increase2} increases the index into the action point list which changes the assumes until the last one which then places no restriction on the encoding. By construction, the encoding can use all $D_{max}$ action points when no assumptions are present.
