# Supplementary material for: SMT-Based Dynamic Multi-Robot Task Allocation
Source: arXiv:2403.11737 source file (2024-03-18)
Supplement: Supplementary file 2 [file sketch_appendix.tex]

\section{Theoretical Results} \label{sec:theoretical}
Some proofs and proof sketches have been removed from the main text due to space considerations. Further theoretical results can be found at \url{http://tinyurl.com/NFM2024-DynamicMRTA}. We assume the solver used is sound and complete for the theories of bitvectors, uninterpreted functions, and linear integer arithmetic.

\begin{lemma}
    \textbf{Consistency of action sequences.} If $result_0$ is sat, $\plan_0 \models \allconsistentpredicate$.
\end{lemma}

\begin{proof}
    (Sketch) Plan building is deterministic, so per assignment, we will only get one possible $\plan_0$. We argue that action point times are strictly monotonically increasing. Because the task start and end literals can only be assigned one time, they can only be assigned one action point, so pick and drop actions occur once. For load constraints, we connect the load of an action sequence to the load at each action point and can say that is constrained by construction. Other aspects are true by construction.
\end{proof}

\begin{lemma}
    \textbf{Completion of tasks.} If $result_0$ is sat, $\plan_0 \models \allcompletedpredicate$ for $\taskset = \taskset_0$.
\end{lemma}

\begin{proof}
    (Sketch) By Lemma \ref{lemma:consistent_action_seq}, we know each agent's action sequence is consistent. By construction, each task must be assigned an agent id and will only be assigned one agent because agent ids are unique. An assignment implies that an agent starts (picks up) the task which implies the agent also ends (drops) the task. The duration of every pick or drop element in the action sequence is equal to the time of a corresponding action point. With this we show the duration constraints are satisfied.
\end{proof}

\begin{lemma}
    \textbf{Plans are updated.} Assume $result_j$ is sat. If $result_{j+1}$ is sat, $\plan_{j+1} \models \updatedpredicate[\plan_j]$
\end{lemma}

\begin{proof}
    (Sketch) For each agent, action sequences are constructed deterministically from an assignment. $\modeloutput_{j+1}$ is constrained to have $\dptuple = \modeloutput_j(\dptuple)$ $\forall d = 1, \ldots, d'-1$ for some $d' = 1, \ldots, D$. Thus, some length prefix in each action sequence is equivalent. In SavePastState(), we either add constraints until the end of the relevant action points ($d + 1 < D \wedge \nextdpid = n$), making the new prefix equal to the old after which we add a wait by construction. In the other, we continue until the time of the action point is $\geq t_j$, which will satisfy the other option for an updated plan. By construction, the last action will be a pick or a drop.
    \iffalse
    \begin{itemize}
        \item 1-to-1 translation from dp times to durations
        \item each point is saved before checking if the time is past the output value unless the next point signifies a wait
        \item if a wait is needed, it will be adhered to based on (E.6) because $t_j$ will be greater than $\prevdptime$
    \end{itemize}
    \fi
\end{proof}

\begin{lemma}
    \textbf{Updated consistency.} Assume $result_j$ is sat. If $result_{j+1}$ is sat, $\plan_{j+1} \models \allconsistentpredicate$.
\end{lemma}

\begin{proof}
    (Sketch) The statements from the proof of Lemma \ref{lemma:consistent_action_seq} hold except that a wait action can now exist. $\wait \cap \move = \emptyset$, so there will still not be two adjacent moves. The addition of a wait either shifts both pick and drop points for a task or shifts just the drop, so drop will still be after pick. Waits are not directly included in the action point encoding, so times are still unique. Therefore, pick and drop actions still only occur once. Similarly, waits will not affect the load values of the action points.
    \iffalse
    \begin{itemize}
        \item We know from above that initial solve is Sat
        \item Save past state is saving a prefix of the sequence which will also be consistent
        \item Similar argument other than load does not start at 0.
    \end{itemize}
    \fi
\end{proof}

\begin{lemma}
    \textbf{Updated completion.} Assume $result_j$ is sat. If $result_{j+1}$ is sat, $\plan_{j+1} \models \allcompletedpredicate$ where $\taskset =(\bigcup_{j'=0}^{j+1} \taskset_{j'})$.
\end{lemma}

\begin{proof}
    (Sketch) We know by Lemma \ref{lemma:updated_consistency} that the updated action sequence is consistent. The statements in Lemma \ref{lemma:completed_tasks} hold for the new set of tasks.  
\end{proof}

\begin{theorem}
    \textbf{Soundness of Algorithm.} Algorithm \ref{alg:overall} is sound.
\end{theorem}

\begin{proof}
     (Sketch) Assuming $result_0 = sat$, the initial plan $\plan_0 \models \updatedpredicate[\emptyset]$ by definition. By Lemmas \ref{lemma:consistent_action_seq} and \ref{lemma:completed_tasks}, $\plan_0 \models \allconsistentpredicate \wedge \allcompletedpredicate$. In order to make an inductive argument for soundness, we need to show for $j>1$ that $(result_{j-1} = sat \Rightarrow \plan_{j-1}$ is valid and updated) $\Rightarrow (result_{j} = sat \Rightarrow \plan_{j}$ is valid and updated). We have two cases: 1) $result_{j-1} = sat$ and 2) $result_{j-1} \neq sat$. By construction, the algorithm will end and return unsat if $result_{j-1} \neq sat$ for $j>0$, so if $(result_{j-1} = sat \Rightarrow \plan_{j-1}$ is valid and updated) $\wedge\ (result_j \neq sat)$ then $result_{j-1} \neq sat$ for $j>0$ proving the statement for this case. For $j>0$, if we assume $(result_{j-1} = sat \Rightarrow \plan_{j-1}$ is valid and updated) $ \wedge\ result_{j-1}$ is sat, by Lemmas \ref{lemma:updated_plans}, \ref{lemma:updated_consistency}, and \ref{lemma:updated_completion}, $result_{j} = sat$ implies $\plan_j$ is an updated, valid plan. Therefore, by induction, for any for any $j$, $result_j = sat$ implies $\plan_j$ is a valid, updated plan.
\end{proof}

\iffalse
\begin{lemma}
    Algorithm \ref{alg:overall} is complete with respect to a given number of action points.
\end{lemma}

\begin{proof}
    Should be more or less the proof below.
\end{proof}
\fi

\begin{lemma}
    \textbf{Maximum number of action points} If an assignment $\modeloutput$ does not exist for an encoding $\encoding$ when $D = D_{max} = 2\numtasks + 1$ of action points then no assignment $\modeloutput$ exists for $D > D_{max}$. 
\end{lemma}

\begin{proof}
    (Sketch) As shown in Lemma \ref{lemma:consistent_action_seq}, pick and drop ids will only occur once per task in an agent's assignment in a satisfying $\modeloutput$. By construction, action point ids must be either $\dpid = \agent$ or $\dpid \geq \numagents \wedge \dpid < 2\numtasks + \numagents$. Therefore, for an agent $\agent$, the maximum number of action points that can be assigned to a value other than $\agent$ is $2\numtasks$. Adding in the constrained 0th action point, the total is $2\numtasks + 1 = D_{max}$ where $\dpid = n$ for $d = d' \geq D_{max}$. By construction $\dptime[\agent][d']=max\_time$ and $\dpload[\agent][d'] = 0$ because picked up tasks must have been dropped off beforehand. Therefore, adding an extra action point does not add new free variables, so an unsat result cannot turn sat by adding more action points.
\end{proof}

\begin{lemma}
    Assume $\Gamma[|\dplist| -1]$. If $D=D_{max}$ algorithm, \ref{alg:overall} is complete.
\end{lemma}

\begin{proof}
    (Sketch) We show this by proving the contrapositive "if a valid, updated plan $\plan_{j+1}$ exists from a previous valid plan $\plan_j$ then we can find a satisfying assignment $\modeloutput$". Taking $\plan_{j+1}$, for each agent, we find the 1-indexed subsequence of indices of pick and drop actions. For each element $k$ in the subsequence, let $\dpid[\agent][k] = 2\mu + \numagents$ where $\mu$ is the number of the task that is picked or dropped, $\dptime[\agent][k] = \duration(\sequenceelement[k])$, and $\dpload[\agent] = \sequenceload_k(\sequenceelement[k])$ until $\duration(\sequenceelement[k+1]) > \tasksetarrivaltime$. Then, remove any wait ($\wait$) actions from the rest of the sequence, adjusting the subsequence of indices accordingly. Continue adding action points for the rest of the indices. Set all remaining action points to $(\agent, max\_time, 0)$. It can be shown that this assignment is satisfying by going through each constraint in the encoding.
\end{proof}

\begin{lemma}
    Following Algorithm \ref{alg:overall}, k will eventually be such that the number of free action points $D = D_{max}$.
\end{lemma}

\begin{proof}
    (Sketch) An action point $d$ is free if it is not constrained to have $\dpid = \agent$.  By inspection we see that the while loop in Lines \ref{line:dp_increase1} and \ref{line:dp_increase2} increases the index into the action point list which changes the assumes until the last one which then places no restriction on the encoding. By construction, the encoding can use all $D_{max}$ action points when no assumptions are present.
\end{proof}

\iffalse
\begin{lemma}
    Following Algorithm \ref{alg:overall}, if a solution exists for a given number of action points, a solution exists if that number is incrementally reached.
\end{lemma}

\begin{proof}
    (Sketch) The constraints are the same in both cases. We probably need an argument here that the approach is complete for a given number of action points as well.
\end{proof}
\fi

\begin{theorem}
    \textbf{Completeness of Solve.} Algorithm \ref{alg:overall} is complete.
\end{theorem}

\begin{proof}
    (Sketch) By Lemma \ref{lemma:incr_to_max}, we will reach $\numdp = D_{max}$. By Lemma \ref{lemma:complete_given_max}, we know that given a sufficiently large $\numdp = D_{max}$, the algorithm is complete.
\end{proof}
